# Supplementary material for: An Improved Data Assimilation Scheme for High Dimensional Nonlinear Systems
Source: arXiv:1208.0065 source file (2012-08-01)
Supplement: Supplementary file 1 [file appendix_A.tex]

\section*{ Appendix A} \label{apx:A}
Suppose a pdf is approxmated by:

\begin{equation}
p(\bx) = \sum_{i = 1}^{l} \alpha_i \  N(\bx - \bx_i , \Sigma_i)
\end{equation}    
when \[ \sum_{i = 1}^{l} \alpha_i = 1.0\]
Then the mean and covariance matrix is obtained as:
\begin{eqnarray*}
E\lbrace \bx \rbrace \equiv \bar{\bx} &=& \int_{-\infty}^{\infty} \bx  p(\bx) \ d\bx \\
& = & \int_{-\infty}^{\infty} \bx  \sum_{i = 1}^{l} \alpha_i \  N(\bx - \bx_i , \Sigma_i) \ d\bx \\
& = &  \sum_{i = 1}^{l} \alpha_i \int_{-\infty}^{\infty} \bx  \  N(\bx - \bx_i , \Sigma_i) \ d\bx \\
& = & \sum_{i = 1}^{l} \alpha_i \bx_i
\end{eqnarray*}

\begin{eqnarray*}
E\lbrace{  (\bx - \bar{\bx})(\bx - \bar{\bx})^T \rbrace} &=& \int_{-\infty}^{\infty} (\bx - \bar{\bx})(\bx - \bar{\bx})^T  p(\bx) \ d\bx \\
&=&\int_{-\infty}^{\infty} (\bx - \bar{\bx})(\bx - \bar{\bx})^T \sum_{i = 1}^{l} \alpha_i \  N(\bx - \bx_i , \Sigma_i) \ d\bx \\
&=& \sum_{i = 1}^{l} \alpha_i^a \int_{-\infty}^{\infty} (\bx - \bar{\bx})(\bx - \bar{\bx})^T   N(\bx - \bx_i , \Sigma_i) \ d\bx \\
&=& \sum_{i = 1}^{l} \alpha_i^a \int_{-\infty}^{\infty} ([\bx - \bx_i] + [\bx_i - \bar{\bx}])([\bx - \bx_i] + [\bx_i - \bar{\bx}])^T   N(\bx - \bx_i , \Sigma_i) \ d\bx \\
&= & \sum_{i = 1}^{l} \alpha_i \Sigma_i + \sum_{i = 1}^{l} \alpha_i (\bx_i - \bar{\bx})^2
\end{eqnarray*}

\subsection{EnKF update equation}
move state without perturbing observations
\begin{eqnarray}
A_1^a = A^f + K (\bar{D} - H A^f) \\
\bar{A_1^a} = \bar{A^f} + K (\bar{D} - H \bar{A^f}) \\
A_1'^a = (I- K H) A'^f
\end{eqnarray}

move the mean with different observations:
\begin{eqnarray}
A_2^a = \bar{A^f} + K (D - H A^f) \\
\bar{A_2^a} = \bar{A^f} + K (\bar{D} - H \bar{A^f}) \\
A_2'^a = K D'
\end{eqnarray}

Final ensemble :
\begin{eqnarray}
A^a = \bar{A^a}  + A_1'^a + A_2'^a \\
A^a = \left( \bar{A^f} + K (\bar{D} - H \bar{A^f}) \right) + \left(A'^f + K (D' - H A'^f) \right) 
\end{eqnarray}
note that
\begin{equation}
\bar{A^a} = \bar{A_1^a} = \bar{A_2^a}
\end{equation}

compared to Burger et al. :

Burger:
\begin{equation}
\bar{A^a} = A^f + K (D - H A^f)
\end{equation}
Monajemi:
\begin{equation}
\bar{A^a} = \left( \bar{A^f} + K (\bar{D} - H \bar{A^f}) \right) + \left(A'^f + K (D' - H A'^f) \right) 
\end{equation}
